# Supplementary material for: Anomalous Diffusion and Emergent Universality in Coupled Memory-Driven Systems
Source: arXiv:2411.09092 source file (2025-08-22)
Supplement: Supplementary file 1 [file suppl.pdf]

# Supplementary Material for "Anomalous Diffusion and Emergent Universality in Coupled Memory-Driven Systems"

Nick Dashti,[1,2,*] M. N. Najafi,[3] and Debra J. Searles[1,4,5,†]

[1] *Australian Institute of Bioengineering and Nanotechnology, The University of Queensland, Brisbane, QLD, 4072, Australia*

[2] *School of Chemistry, University of Melbourne, Melbourne, Victoria 3010, Australia*

[3] *Department of Physics, University of Mohaghegh Ardabili, P.O. Box 179, Ardabil, Iran*

[4] *School of Chemistry and Molecular Biosciences, The University of Queensland, Brisbane, QLD, 4072, Australia*

[5] *ARC Centre of Excellence for Green Electrochemical Transformation of Carbon Dioxide, The University of Queensland, Brisbane, QLD, 4072, Australia*

This supplemental material contains:

- Pseudo-code: simulation algorithm for coupled agent model
- Mean-squared displacement $R_t^2$: 1D pheromonal random walk
- Mean-squared distance $D_t^2$: 1D pheromonal random walk
- Mean-squared increment $\Delta_{t,T}^2$: 1D pheromonal random walk
- Position probability distribution $P(x,t)$: 1D pheromonal random walk
- Distance probability distribution $P(D,t)$: 1D pheromonal random walk
- Probability distribution of encounters $P(m,t)$ and $P(\mathcal{T},t)$: 1D normal random walk ($\beta = 0, \beta' = 0$)
- Probability distribution of encounters $P(m,t)$: 1D pheromonal random walk
- Mean-squared displacement $R_t^2$: 2D pheromonal random walk
- Mean-squared increment $\Delta_{t,T}^2$: 2D pheromonal random walk
- Position probability distributions $P(x, y=0, t)$ and $P(x=0, y, t)$: 2D pheromonal random walk
- Probability distribution of encounters $P(m,t)$ and $P(\mathcal{T},t)$: 2D normal random walk ($\beta = 0, \beta' = 0$)
- Probability distribution of encounters $P(m,t)$: 2D pheromonal random walk

* dashti.nick@gmail.com

† d.bernhardt@uq.edu.au

## Pseudo-code

The following pseudo-code outlines the simulation algorithm used to model the coupled dynamics of two pheromone-guided agents as described in the main manuscript.

Initialize pheromone fields: $h_i^A \leftarrow 0$, $h_i^B \leftarrow 0$ for all sites $i$
Set initial positions: $x_0^A \leftarrow 0$, $x_0^B \leftarrow D_0$
**for** $t = 1$ to $t_{\max}$ **do**
    **for** each agent $X \in \{A, B\}$ **do**
        Let $i = x_{t-1}^X$
        Compute transition probabilities $p_{i\to j}^X$ to the nearest neighbors $j \in \mathrm{nn}(i)$ using the pheromone fields at time step $t-1$
    **end for**
    Sample new positions $x_t^A$, $x_t^B$ from the computed probabilities
    **for** each agent $X \in \{A, B\}$ **do**
        Let $i = x_t^X$
        **if** $i$ exceeds the current bounds of $h^X$ **then**
            Enlarge $h^X$ and redefine its domain to cover $i$; initialize new entries to 0
        **end if**
        Update pheromone field: $h_i^X \leftarrow h_i^X + 1$
    **end for**
**end for**

**Note on Implementation:** In the simulation, the pheromone fields $h^A$ and $h^B$ are conceptually treated as arrays indexed by site positions. However, since the system is open, agents can explore arbitrarily large distances from the origin, especially in cases where the self-avoiding coefficient $\beta$ dominates. This can result in extremely large array sizes and high memory usage. To address this, we implement $h^A$ and $h^B$ as hash tables (e.g., using the `std::unordered_map` class in C++), which allows for efficient, sparse storage of only the sites visited by each agent. This approach significantly reduces memory usage while maintaining correct model behavior. The hash table method is particularly efficient for systems in spatial dimensions $d > 1$, where a large number of lattice sites remain unvisited.

## Supplementary Figures

The following figures provide additional results from the numerical simulations described in the main manuscript, including key observables such as mean-squared displacement, inter-agent distances, and probability distributions for both 1D and 2D pheromonal random walks.

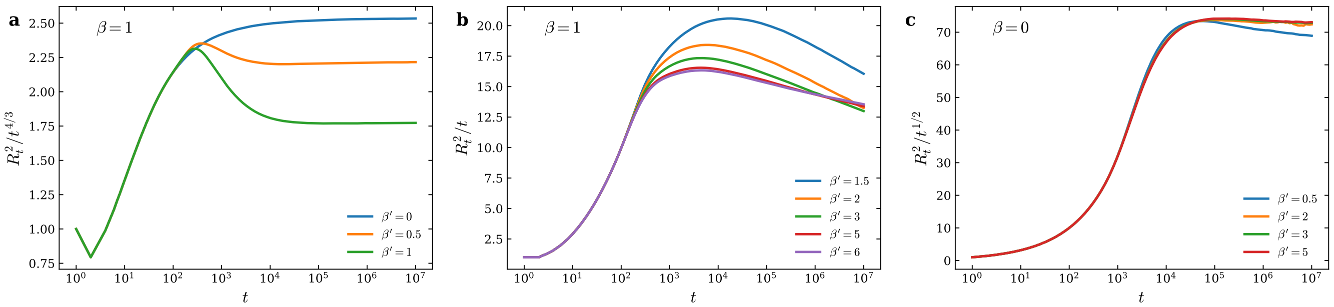


Fig S1. **Mean-squared displacement for 1D pheromonal random walk.** (a) $R_t^2 \sim t^{4/3}$ for $\beta' \leq \beta$, where $\beta = 1$. (b) $R_t^2 \sim t^{1^-}$ for $\beta' > \mathcal{B}$, where $\beta = 1$. (c) $R_t^2 \sim t^{1/2}$ for $\beta' > \mathcal{B}$, where $\beta = 0$.

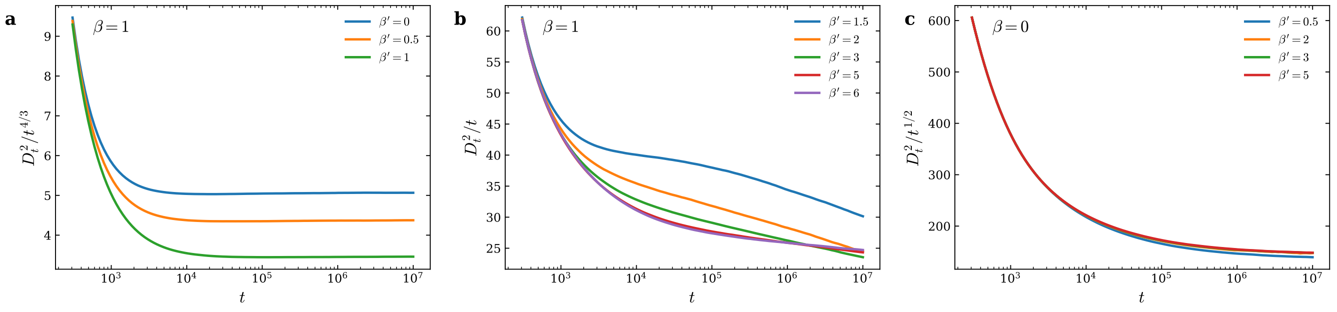


Fig S2. **Mean-squared distance between random walks for 1D pheromonal random walk.** (a) $D_t^2 \sim t^{4/3}$ for $\beta' \leq \beta$, where $\beta = 1$. (b) $D_t^2 \sim t^{1^-}$ for $\beta' > \mathcal{B}$, where $\beta = 1$. (c) $D_t^2 \sim t^{1/2}$ for $\beta' > \mathcal{B}$, where $\beta = 0$.

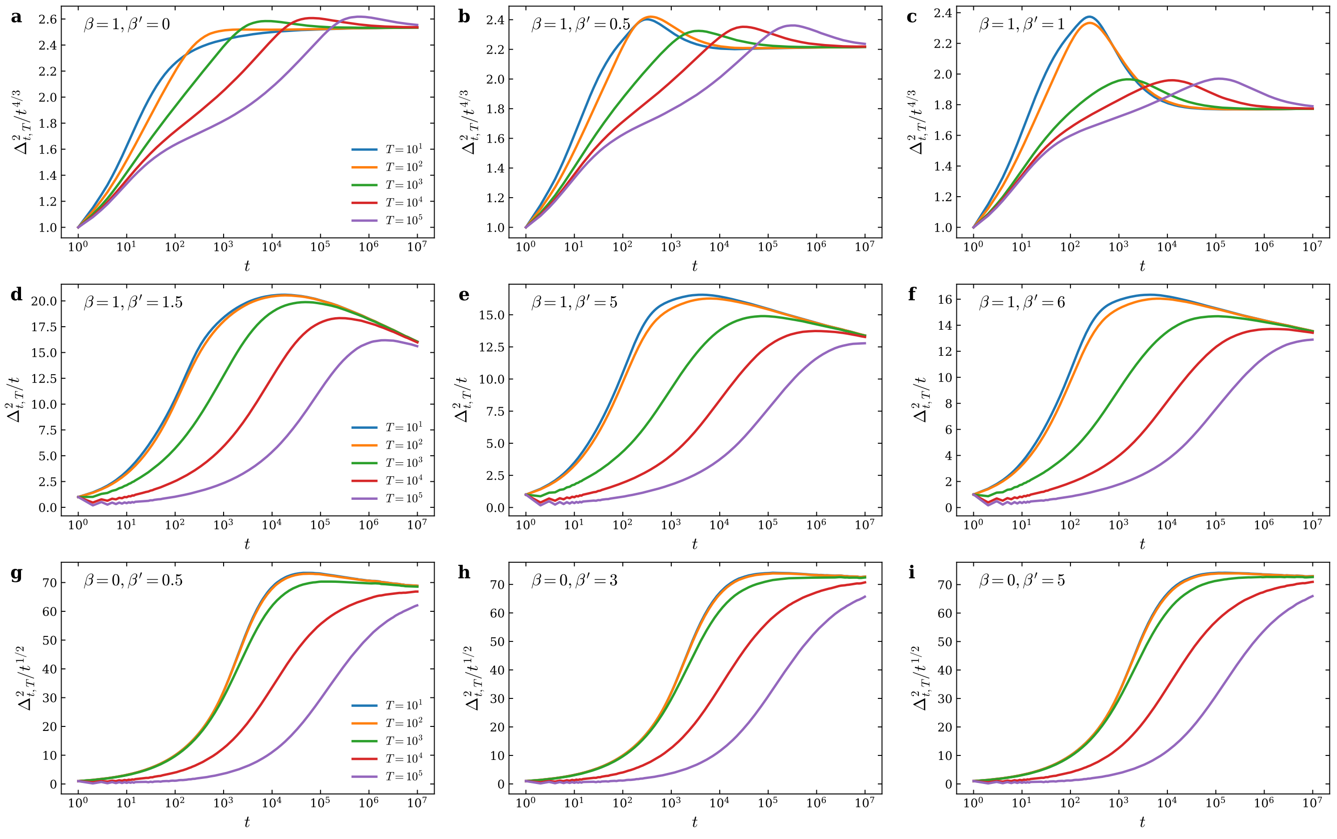


Fig S3. **Mean-squared increment for 1D pheromonal random walk.** (a)-(c) $\Delta^2_{t,T} \sim t^{4/3}$ for $\beta' \leq \beta$, where $\beta = 1$. (d)-(f) $\Delta^2_{t,T} \sim t^{1^-}$ for $\beta' > \mathcal{B}$, where $\beta = 1$. (g)-(i) $\Delta^2_{t,T} \sim t^{1/2}$ for $\beta' > \mathcal{B}$, where $\beta = 0$.

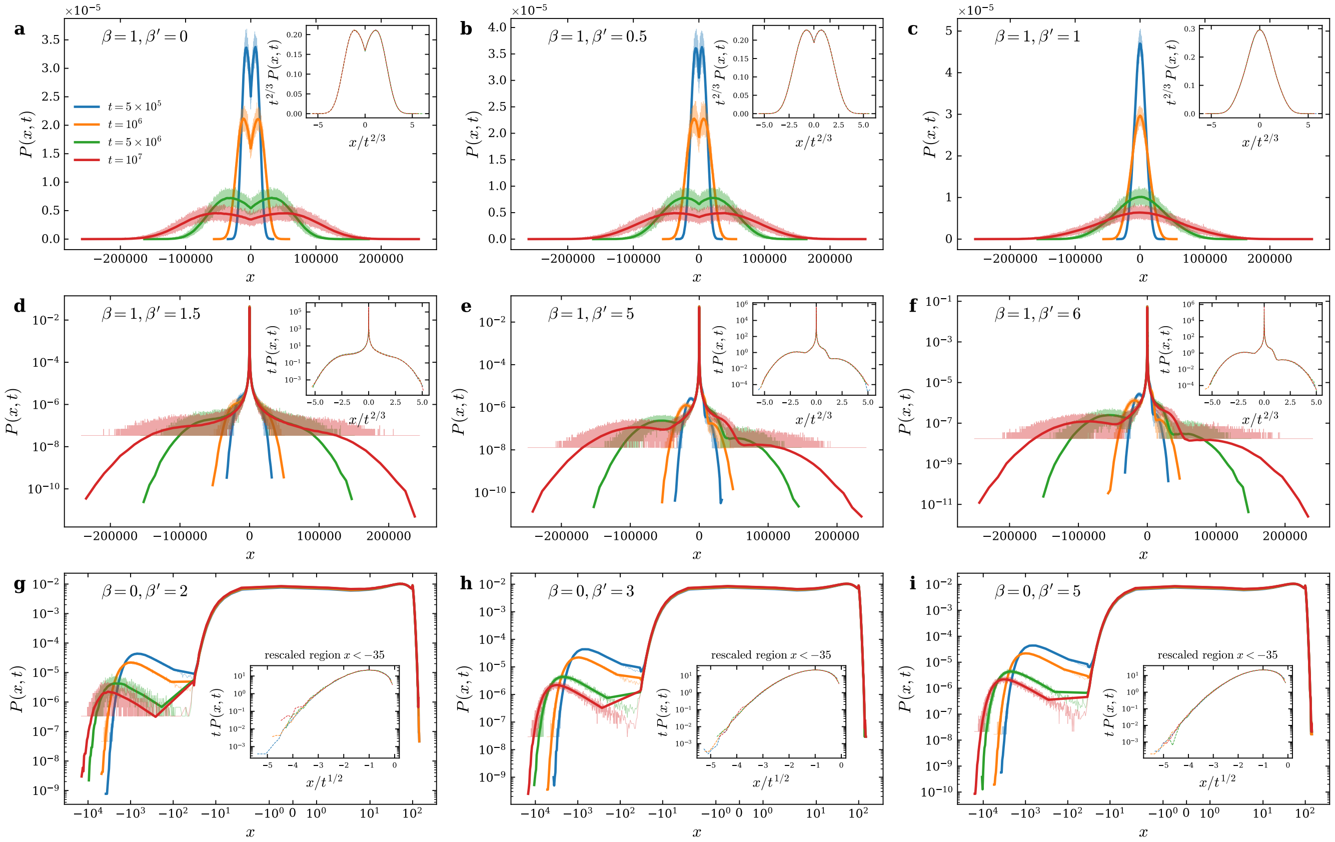


Fig S4. **Position probability distribution for 1D model** (a)-(c) Thin-tailed position distributions for $\beta' \leq \beta$. The collapse scaling relation is $x \to x/t^{2/3}$ and $P \to t^{2/3}P$. (d)-(f) Fat-tailed position distribution for $\beta' > \mathcal{B}$. The collapse scaling relation is $x \to x/t^{2/3}$ and $P \to tP$. (g)-(i) Fat-tailed position distribution for $\beta' > \mathcal{B}$, when $\beta = 0$. The collapse scaling relation for the region $x \lessapprox -35$ is $x \to x/t^{1/2}$ and $P \to tP$.

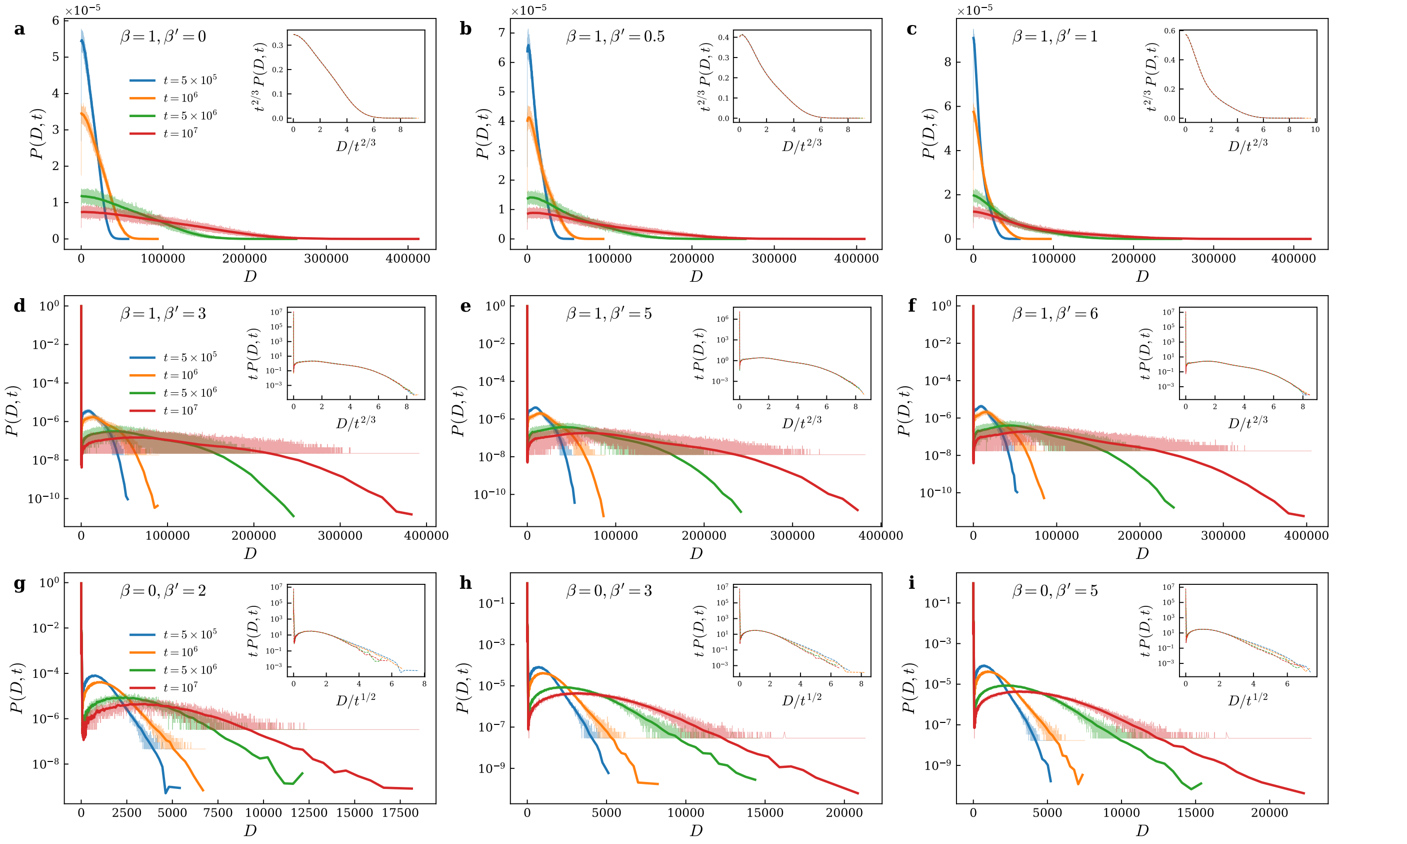


Fig S5. **Distance probability distribution for 1D model** (a)-(c) Thin-tailed distributions for $\beta' \leq \beta$. The collapse scaling relation is $D \to D/t^{2/3}$ and $P \to t^{2/3}P$. (d)-(f) Fat-tailed position distribution for $\beta' > \mathcal{B}$. The collapse scaling relation is $D \to D/t^{2/3}$ and $P \to tP$. (g)-(i) Fat-tailed position distribution for $\beta' > \mathcal{B}$, when $\beta = 0$. The collapse scaling relation is $D \to D/t^{1/2}$ and $P \to tP$.

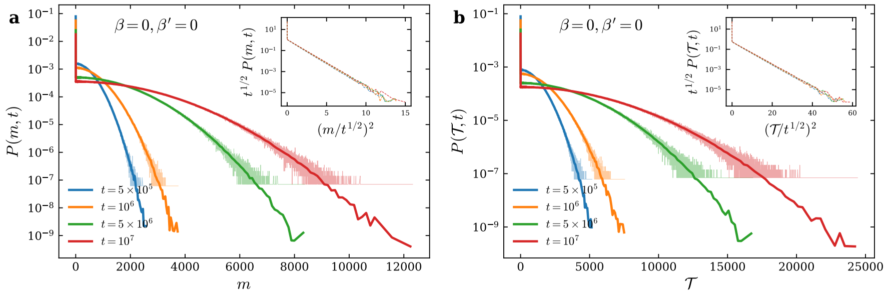


Fig S6. **Probability distribution of encounters for 1D normal random walks.** For the model with $\beta = 0, \beta' = 0$, the distributions of mating frequency ($m$) and total mating duration ($\mathcal{T}$) exhibit Gaussian behavior and collapse under the scaling relations $m \to m/t^{1/2}$, $\mathcal{T} \to \mathcal{T}/t^{1/2}$ and $P \to t^{1/2}P$.

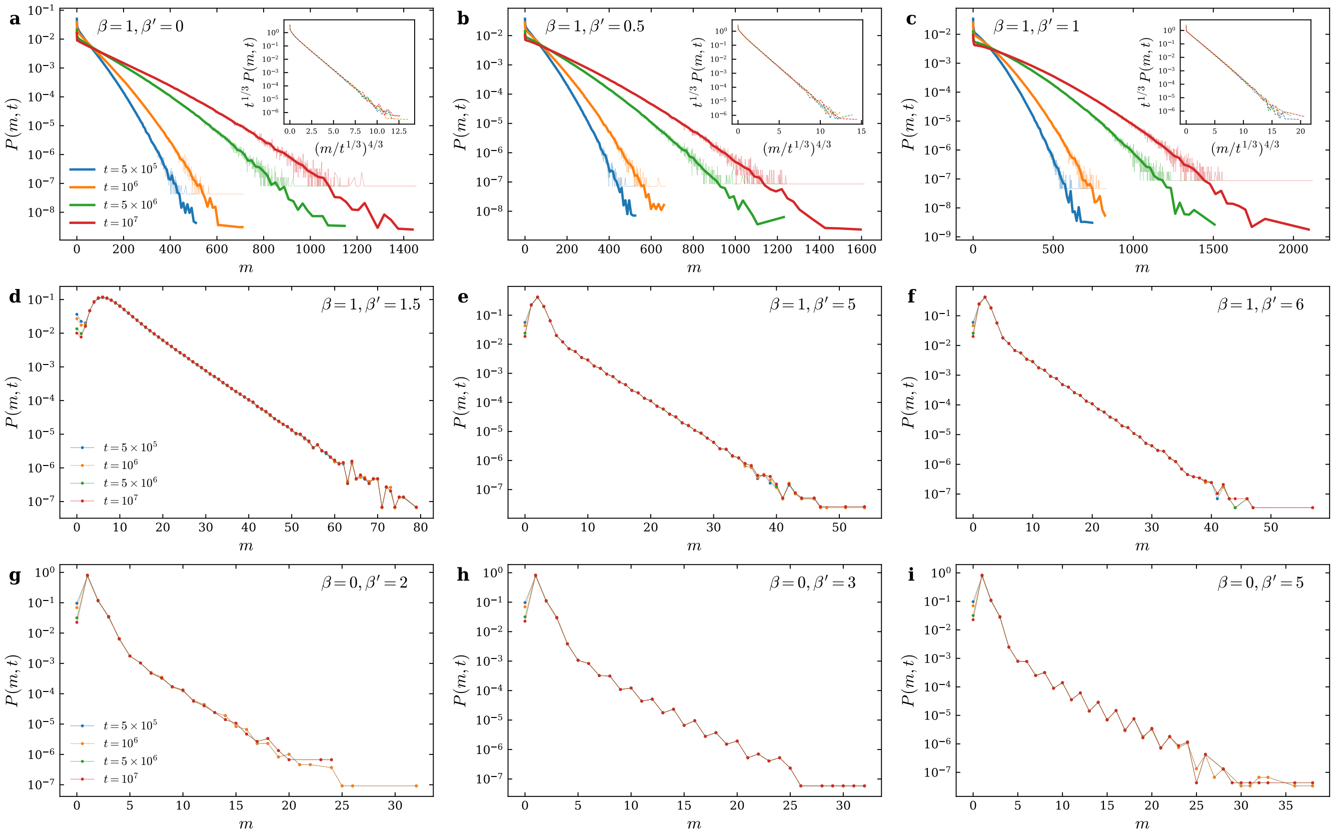


Fig S7. **Probability distribution of encounters for 1D pheromonal random walk** (a)-(c) Tail of all distributions exhibit compressed exponential behavior of the form $\exp(-z^{4/3})$ and collapse under the scaling relations $m \to m/t^{1/3}$ and $P \to t^{1/3} P$. (d)-(i) The tail of the distribution $P(m, t)$ follows an exponential decay, $\exp(-m)$, and is time-independent.

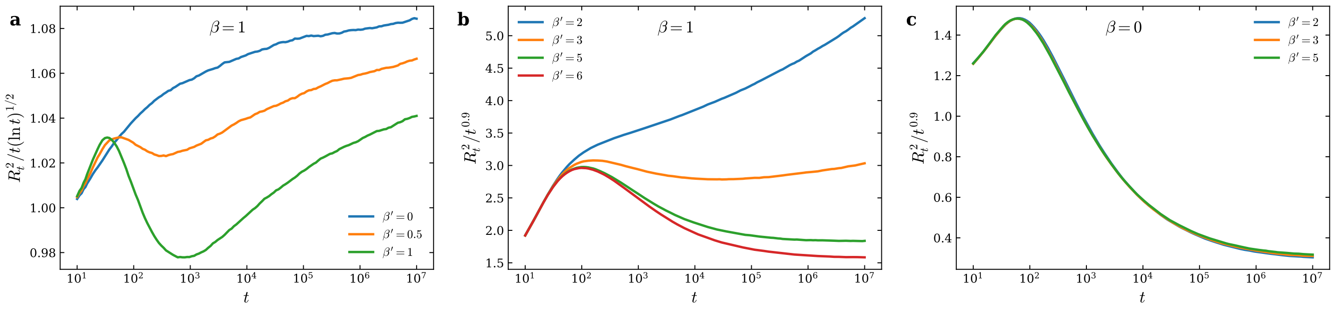


Fig S8. **Mean-squared displacement for 2D pheromonal random walk.** (a) $R_t^2 \sim t(\ln t)^{1/2}$ for $\beta' \le \beta$. (b)-(c) $R_t^2 \sim t^{0.9}$ for $\beta' > \mathcal{B}$.

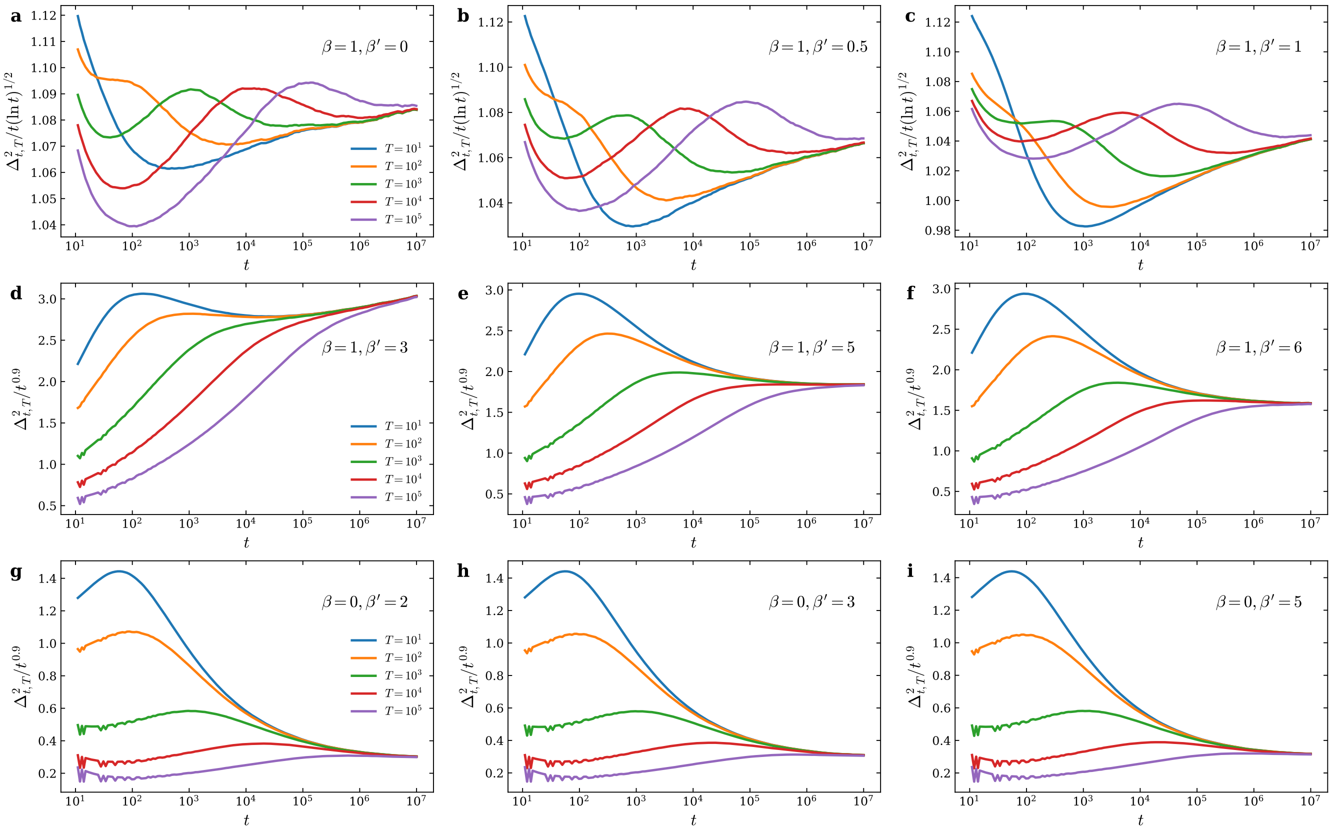


Fig S9. **Mean-squared increment for 2D pheromonal random walk.** (a)-(c) $\Delta^2_{t,T} \sim t(\ln t)^{1/2}$ for $\beta' \leq \beta$. (d)-(i) $\Delta^2_{t,T} \sim t^{0.9}$ for $\beta' > \mathcal{B}$.

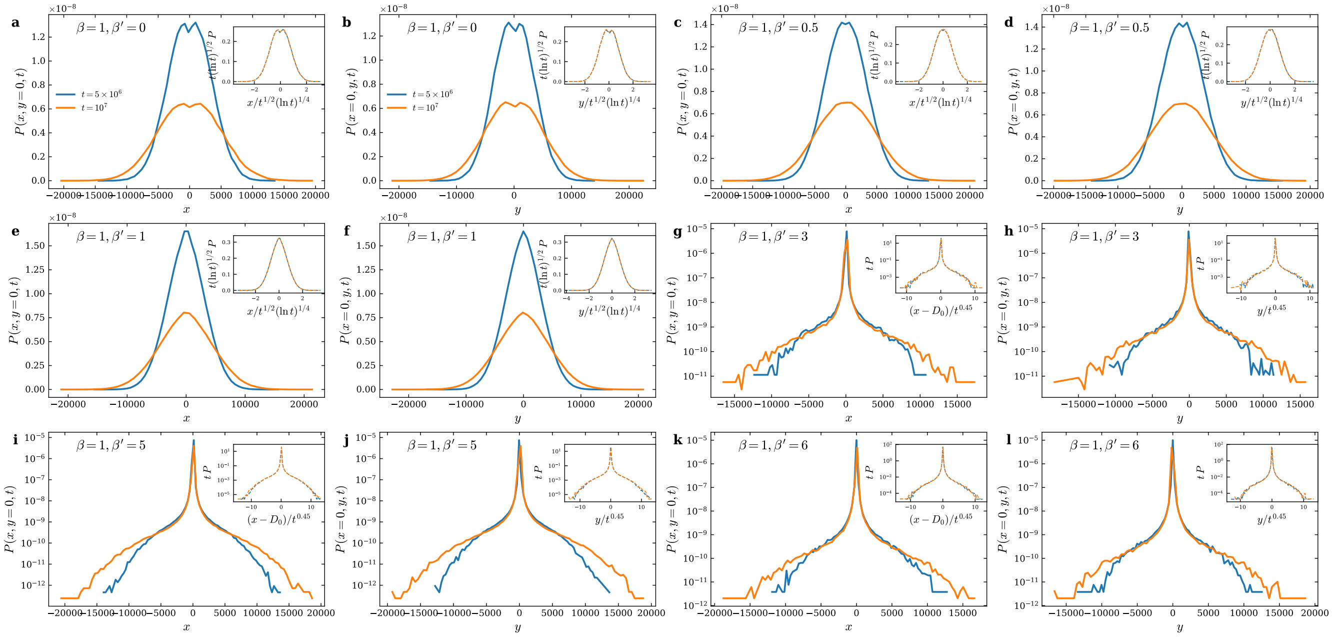


Fig S10. **Position probability distribution for 2D pheromonal random walk** (a)-(f) Thin-tailed distributions for $P(x, y = 0, t)$ and $P(x = 0, y, t)$ when $\beta' \leq \beta$. The collapse scaling relation is $(x, y) \to (x, y)/t^{1/2}(\ln t)^{1/4}$ and $P \to t(\ln t)^{1/2}P$. (g)-(l) Fat-tailed distribution for $P(x, y = 0, t)$ and $P(x = 0, y, t)$ when $\beta' > \mathcal{B}$. The collapse scaling relation is $(x, y) \to (x - D_0, y)/t^{0.45}$ and $P \to tP$.

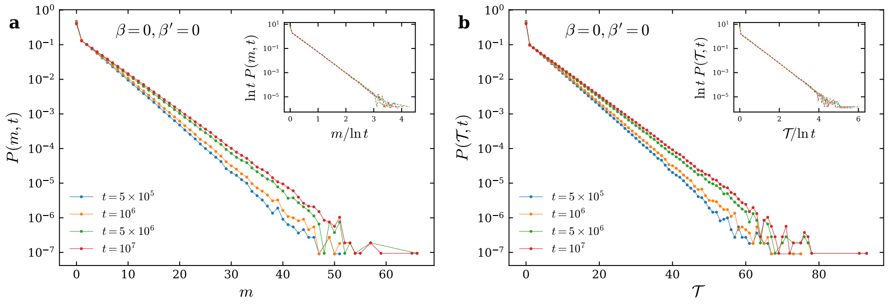


Fig S11. **Probability distribution of encounters for 2D pheromonal random walk.** For the model with $\beta = 0, \beta' = 0$, the distributions of mating frequency ($m$) and total mating duration ($\mathcal{T}$) exhibit exponential behavior and collapse under the scaling relations $m \to m/\ln t$, $\mathcal{T} \to \mathcal{T}/\ln t$ and $P \to (\ln t)P$.

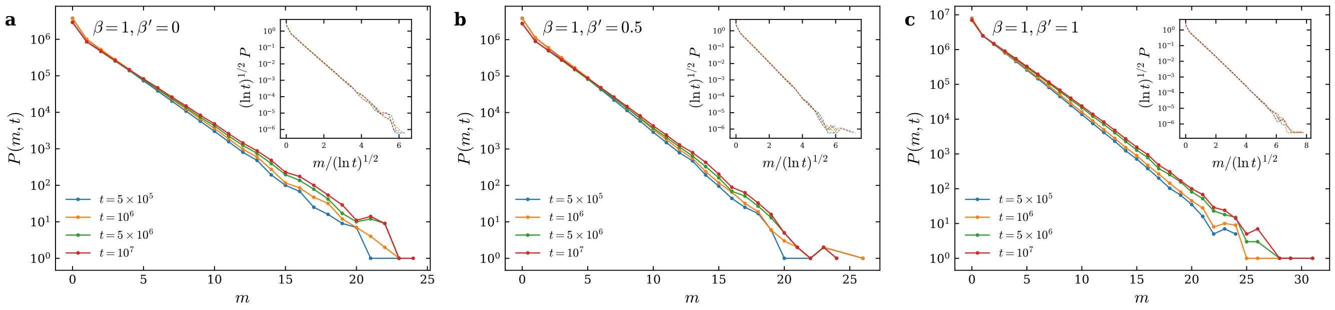


Fig S12. **Probability distribution of encounters for 2D pheromonal random walk.** (a)-(c) For $\beta' \leq \beta$, the mating frequency distributions follow the relation $\exp(-z)$ and the curves collapse under the transformations $m \to m/(\ln t)^{1/2}$ and $P \to (\ln t)^{1/2}P$, respectively.
